# Supplementary material for: Job Dispatching Policies for Queueing Systems with Unknown Service Rates
Source: arXiv:2106.04707 source file (2021-06-10)
Supplement: Supplementary file 1 [file appendix.tex]

\section{Appendix} \label{appendix}
\begin{enumerate}
    \item \textit{Proof of expression for optimal $p_i^*$[\ref{optimal_p}]}\label{prf_optimal_p}
    For a a discrete time queueing system with arrival according $Ber(\lambda)$ and departure according $Ber(\mu)$, the mean queue length is given by 
    \begin{equation}
        \expectation[\queue] = \frac{\rho}{1-\rho}
    \end{equation}
    where $\rho = \frac{\lambda(1- \mu)}{\mu(1-\lambda)}$. So if we send each incoming job to server $i$ according to probability $p_i$. the mean queue length is given by
    \begin{equation}\label{rel:opt_eqn}
        \expectation[\queue_{system}] = \expectation\left[\sum_i\queue_i\right] = \sum_i \frac{\rho_i}{1-\rho_i} = \sum_i \frac{\lambda p_i(1 - \mu_i)}{\mu_i - \lambda p_i}.
    \end{equation}
    Notice, this is the exact term we wanted minimize in the optimization problem. To ensure that the individual queues are stable $\lambda p_i \leq \mu_i, \> \forall i$ is required. Also, to ensure that each job is sent to some server $\sum_i p_i = 1$ is required. These were constraints of the optimization problem along with the non-negativeness of $p_i, \>\forall i$. Now lagrangian of the optimization problem is given by 
    \begin{equation}
        \mathcal{L} = \sum_i \frac{\lambda p_i(1 - \mu_i)}{\mu_i - \lambda p_i} + a\left(1 - \sum_i p_i\right) + \sum_i b_i\left(\lambda p_i - \mu\right) - \sum_i c_ip_i.
    \end{equation}
    Now 
    \begin{equation}
        \frac{d\mathcal{L}}{d p_i} = \frac{\lambda \mu_i (1-\mu_i)}{(\mu_i - \lambda p_i)^2} - a + b_i\lambda - c_i
    \end{equation}
    Since, objective function is convex, inequality constraints are convex and equality constraint is affine, the dual gap is zero. From complementary slackness
    \begin{equation}
        c_i^* p_i^* = 0
    \end{equation}
    \begin{equation}
        b_i^* (\lambda p_i^* - \mu_i) = 0
    \end{equation}
    Since, $\lambda p_i^* < 0, \> \forall i$, $b_i^* = 0, \> \forall i$. Let $\mathbb{S}$ be the set such that $i \in \mathbb{S} \iff p_i^* > 0$. Then $\forall i \in \mathbb{S}$
    \begin{equation}
        \frac{d\mathcal{L}}{d p_i} = \frac{\lambda \mu_i (1-\mu_i)}{(\mu_i - \lambda p_i)^2} - a  = 0
    \end{equation}
    This gives $\forall i$,
    \begin{equation}
        \mu_i - \lambda p_i = a'\sqrt{\mu_i(1-\mu_i)}
    \end{equation}
    where $a' = \sqrt{\frac{\lambda}{a}}$. Summing the above expression for all $i\in \mathbb{S}$, we get
    \begin{equation}
        \sum_{i\in \mathbb{S}} \mu_i - \lambda = a'\left(\sum_{j\in \mathbb{S}}\sqrt{ \mu_j(1-\mu_j)}\right)
    \end{equation}
    Using the value of $a'$ from both the equations, we get
    \begin{align*}
        \frac{\mu_i - \lambda p_i}{\sum_i \mu_i - \lambda} &= \frac{\sqrt{\mu_i(1-\mu_i)}}{\sum_{j\in \mathbb{S}} \sqrt{\mu_j(1-\mu_j)}}\\
        \implies p_i& = \frac{\mu_i}{\lambda} -  \frac{\sqrt{\mu_i(1-\mu_i)}}{\sum_{j\in \mathbb{S}} \sqrt{\mu_j(1-\mu_j)}}\left(\frac{\sum_{i\in \mathbb{S}}\mu_i}{\lambda} - 1\right).
    \end{align*}
    Now, we have the expression, we need to prove that the optimal set is when if $\support^*_i=1 \iff i \in \mathbb{S}$. We will show that all the $3$ conditions of $\support^*$ is required.
    \begin{itemize}
        \item \textit{Requirement of $\ref{rel:support_monotonic}^{st} condition$}\\
        Consider a feasible solution $SOL_1 = p_1, p_2, \cdots, p_\numofserver$ such that there exists $i, j$ such that $p_i< p_j$ and $\mu_i> \mu_j$. Consider another feasible solution $SOL_2$ with the exact same probabilities as $SOL_1$ except the $p_i, p_j$ are interchanged. Now the difference of the value of objective function is given by, 
        \begin{align*}
            &\expectation\left[\queue_{system}_1\right] - \expectation\left[\queue_{system}_1\right] \\
            =& \frac{\lambda p_i (1- \mu_i)}{\mu_i - \lambda p_i} + \frac{\lambda p_j (1- \mu_j)}{\mu_j - \lambda p_j} - \frac{\lambda p_j (1- \mu_i)}{\mu_i - \lambda p_j} - \frac{\lambda p_i (1- \mu_j)}{\mu_j - \lambda p_i}\\
            =&\lambda p_j\frac{(\mu_i - \mu_j)(1-\lambda p_j)}{(\mu_j - \lambda p_j)(\mu_i - \lambda p_j)} + \lambda p_i\frac{(\mu_j - \mu_i)(1-\lambda p_i)}{(\mu_i - \lambda p_i)(\mu_j - \lambda p_i)}\\
            =&\lambda \left(\mu_i - \mu_j\right) \left(p_j - p_i\right)\left(\frac{\mu_i\mu_j + \lambda^2 p_i p_j(\mu_i + \mu_j) - \lambda^2 p_ip_j - \lambda\mu_i\mu_j(p_i + p_j)}{(\mu_i - \lambda p_i)(\mu_j - \lambda p_i)(\mu_j - \lambda p_j)(\mu_i - \lambda p_j)}\right)\\
            =& \frac{\lambda\left(\mu_i - \mu_j\right) \left(p_j - p_i\right)}{(\mu_i - \lambda p_i)(\mu_j - \lambda p_i)(\mu_j - \lambda p_j)(\mu_i - \lambda p_j)}\Big(\left(\mu_i - \lambda p_i\right)\lambda p_i\left(1- \lambda p_i\right) + \left(\mu_j - \lambda p_j\right)\lambda p_j\left(1- \lambda p_j\right) + \\
            &\left(\mu_i - \lambda p_i\right)\left(\mu_j - \lambda p_j\right)\left(\mu_i - \lambda p_i - \lambda p_j\right)\Big)\\
            \geq& 0
        \end{align*}
        where the last inequality is valid since all the terms in the above expression are positive. This means that if $\mu_i \geq \mu_j$, then $\p_i^* \geq p_j^*$. Now $p_i^* >0 \iff i \in \mathbb{S}$. This condition corresponds to $\ref{rel:support_monotonic}^{st}$ property of $\support^*$.
        \item \textit{Requirement of $\ref{rel:support_positive}^{nd} condition$}\\
        A negative probability is not a valid. Hence, the requirement of the condition.
        \item \textit{Requirement of $\ref{rel:support_maximal}^{rd} condition$}\\
        Consider a set $\mathbb{S}'$  such that if $\support_i^* = 0,\> i \notin \mathbb{S}'.$ But $\exists j$ s.t. $j \notin \mathbb{S}'$ but $\support_j^* = 1$. We argue that this is strictly sub-optimal.
        
        When $\mathbb{S}'$ is equivalent to $\mathbb{S}$, then the optimal solution are the probabilities $p_i^*$. However, the feasible set of solutions included all the solution where some of the $p_i$ are fixed to $0$. Notice that when $\exists j$ s.t. $j \notin \mathbb{S}'$ but $\support_j^* = 1$, it corresponds to one of those the feasible solution. Hence, it should be strictly sub-optimal as compared to the optimal solution.
    \end{itemize}
    \item \textit{Proof of lemma \ref{lm_relation_p_mu}}\label{prf_lm_relation_p_mu}\\
    We will use the following set on inequalities.
    \begin{equation}\label{ineq1}
        1 - x \leq \sqrt{1-x} \leq 1 - \frac{x}{2}, \>\> x \in [0, 1]
    \end{equation}
    \begin{equation}\label{ineq2}
        1 + \frac{x}{3} \leq \sqrt{1+x} \leq 1 + x, \>\> x \in [0, 1]
    \end{equation}
    \begin{equation}\label{ineq3}
        1 + x \leq \frac{1}{1 - x}, \>\> x \in [0, 1]
    \end{equation}
    \begin{equation}\label{ineq4}
        \frac{1}{1 - x} \leq 1 + 2x, \>\> x \in [0, \frac{1}{2}]
    \end{equation}
    From the definition of $\Delta$, it is clear that $\lvert\hat{\mu}_i - \mu_i\rvert \leq \Delta,\> \forall i \implies \hat{p}_i = p_i = 0,\> \forall i \notin \mathbb{S}^*$. For any $i \in \mathbb{S}^*$
    \begin{align*}
        \hat{p}_i &= \frac{\hat{\mu}_i}{\lambda} - \frac{\sqrt{\hat{\mu}_i(1-\hat{\mu}_i)}}{\sum_{j\in \mathbb{S}^*}\sqrt{\hat{\mu}_j(1-\hat{\mu}_j)}} \left(\frac{\sum_{j\in \mathbb{S}^*}\hat{\mu}_j}{\lambda} - 1\right)\\
        &\leq \frac{\mu_i + \delta}{\lambda} - \frac{\sqrt{(\mu_i - \delta)(1-\mu_i - \delta)}}{\sum_{j\in \mathbb{S}^*} \sqrt{(\mu_j + \delta)(1 - \mu_j + \delta)}} \left(\frac{\sum_{j\in \mathbb{S}^*}\mu_j - \delta}{\lambda} - 1\right)\\
        &\leq \frac{\mu_i + \delta}{\lambda} - \frac{\sqrt{\mu_i(1-\mu_i)}}{\sum_{j\in \mathbb{S}^*}\sqrt{\mu_j(1-\mu_j)}}\frac{\sqrt{(1 - \frac{\delta}{\mu_i})(1 - \frac{\delta}{1-\mu_i})}}{\sqrt{(1 + \frac{\delta}{\mu_{min}})(1 + \frac{\delta}{1-\mu_{max}})}} \left(\frac{\sum_{j\in \mathbb{S}^*}\mu_j - \delta}{\lambda} - 1\right)\\
        &\overset{(a)}{\leq} \frac{\mu_i + \delta}{\lambda} - \frac{\sqrt{\mu_i(1-\mu_i)}}{\sum_{j\in \mathbb{S}^*}\sqrt{\mu_j(1-\mu_j)}}\frac{(1 - \frac{\delta}{\mu_i})(1 - \frac{\delta}{1-\mu_i})}{(1 + \frac{\delta}{\mu_{min}})(1 + \frac{\delta}{1-\mu_{max}})} \left(\frac{\sum_{j\in \mathbb{S}^*}\mu_j - \delta}{\lambda} - 1\right)\\
        &\overset{(b)}{\leq} \frac{\mu_i + \delta}{\lambda} - \frac{\sqrt{\mu_i(1-\mu_i)}}{\sum_{j\in \mathbb{S}^*}\sqrt{\mu_j(1-\mu_j)}}\left(\frac{\sum_{j\in \mathbb{S}^*}\mu_j}{\lambda} - 1\right)\left(1 - \frac{\delta}{\tilde{\mu}}\right)^4 \left(1 - \frac{\lvert \mathbb{S}^*\rvert \delta}{\sum_{j\in \mathbb{S}^*}\mu_j - \lambda}\right)
    \end{align*}
    where 
    \begin{itemize}
        \item $\tilde{\mu} = \min (\mu_{min}, 1- \mu_{max})$
        \item $(a)$ - Used equation \ref{ineq1}, \ref{ineq2}
        \item $(b)$ - Used equation \ref{ineq3}
    \end{itemize}
    Notice, the above derivation is true if 
    $$\delta \leq \min \left\{\tilde{\mu}, \frac{\epsilon^*}{|\mathbb{S}^*|}\right\}$$
    Hence,
    \begin{align*}
        \hat{p}_i - p_i^* &\leq  \frac{\delta}{\lambda} + \frac{\sqrt{\mu_i(1-\mu_i)}}{\sum_{j\in \mathbb{S}^*}\sqrt{\mu_j(1-\mu_j)}}\left(\frac{\sum_{j\in \mathbb{S}^*}\mu_j}{\lambda} - 1\right)\left(1 - \left(1 - \frac{\delta}{\tilde{\mu}}\right)^4 \left(1 - \frac{\lvert \mathbb{S}^*\rvert \delta}{\sum_{j\in \mathbb{S}^*}\mu_j - \lambda}\right)\right)\\
        &\leq  \frac{\delta}{\lambda} + \left(\frac{\sum_{j\in \mathbb{S}^*}\mu_j}{\lambda} - 1\right)\left(1 - \left(1 - 4\frac{\delta}{\tilde{\mu}}\right) \left(1 - \frac{\lvert \mathbb{S}^*\rvert \delta}{\sum_{j\in \mathbb{S}^*}\mu_j - \lambda}\right)\right)\\
        &\leq  \frac{\delta}{\lambda} + \left(\frac{\sum_{j\in \mathbb{S}^*}\mu_j}{\lambda} - 1\right)\left(\frac{4\delta}{\tilde{\mu}} + \frac{\lvert \mathbb{S}^*\rvert \delta}{\sum_{j\in \mathbb{S}^*}\mu_j - \lambda}\right)\\
        &\leq  \frac{\delta}{\lambda}\left(1 + \frac{4 \epsilon^*}{\tilde{\mu}} + \lvert \mathbb{S}^*\rvert \right)\\
        &\leq  c_1 \delta
    \end{align*}
    where $c_1 = \frac{1}{\lambda}\left(1 + \frac{4 \epsilon^*}{\tilde{\mu}} + \lvert \mathbb{S}^*\rvert \right)$. Similarly,
    \begingroup
    \allowdisplaybreaks
    \begin{align*}
        \hat{p}_i &= \frac{\hat{\mu}_i}{\lambda} - \frac{\sqrt{\hat{\mu}_i(1-\hat{\mu}_i)}}{\sum_{j\in \mathbb{S}^*}\sqrt{\hat{\mu}_j(1-\hat{\mu}_j)}} \left(\frac{\sum_{j\in \mathbb{S}^*}\hat{\mu}_j}{\lambda} - 1\right)\\
        &\geq\frac{\mu_i - \delta}{\lambda} - \frac{\sqrt{(\mu_i + \delta)(1-\mu_i + \delta)}}{\sum_{j\in \mathbb{S}^*} \sqrt{(\mu_j - \delta)(1 - \mu_j - \delta)}} \left(\frac{\sum_{j\in \mathbb{S}^*}\mu_j + \delta}{\lambda} - 1\right)\\
        &\geq \frac{\mu_i - \delta}{\lambda} - \frac{\sqrt{\mu_i(1-\mu_i)}}{\sum_{j\in \mathbb{S}^*}\sqrt{\mu_j(1-\mu_j)}}\frac{\sqrt{(1 + \frac{\delta}{\mu_i})(1 + \frac{\delta}{1-\mu_i})}}{\sqrt{(1 - \frac{\delta}{\mu_{min}})(1 - \frac{\delta}{1-\mu_{max}})}} \left(\frac{\sum_{j\in \mathbb{S}^*}\mu_j + \delta}{\lambda} - 1\right)\\
        &\overset{(a)}{\geq}\frac{\mu_i - \delta}{\lambda} - \frac{\sqrt{\mu_i(1-\mu_i)}}{\sum_{j\in \mathbb{S}^*} \sqrt{\mu_j(1-\mu_j)}} \frac{(1 + \frac{\delta}{\mu_i})(1 + \frac{\delta}{1-\mu_i})}{(1 - \frac{\delta}{\mu_{min}})(1 - \frac{\delta}{1-\mu_{max}})} \left(\frac{\sum_{j\in \mathbb{S}^*}\mu_j + \delta}{\lambda} - 1\right)\\
        &\overset{(b)}{\geq} \frac{\mu_i - \delta}{\lambda} - \frac{\sqrt{\mu_i(1-\mu_i)}}{\sum_{j\in \mathbb{S}^*}\sqrt{\mu_j(1-\mu_j)}}\left(\frac{\sum_{j\in \mathbb{S}^*}\mu_j}{\lambda} - 1\right)\left(1 + \frac{2\delta}{\tilde{\mu}}\right)^4 \left(1 + \frac{\lvert \mathbb{S}^*\rvert \delta}{\sum_{j\in \mathbb{S}^*}\mu_j - \lambda}\right)
    \end{align*}
    \endgroup
    where 
    \begin{itemize}
        \item $\tilde{\mu} = \min (\mu_{min}, 1- \mu_{max})$
        \item $(a)$ - Used equation \ref{ineq1}, \ref{ineq2}
        \item $(b)$ - Used equation \ref{ineq4}
    \end{itemize}
    Notice, the above derivation is true if 
    $$\delta \leq \min \left\{\frac{\tilde{\mu}}{2}, \frac{\epsilon^*}{|\mathbb{S}^*|}\right\}$$
    Hence,
    \begin{align*}
        \hat{p}_i - p_i^* &\geq  -\frac{\delta}{\lambda} + \frac{\sqrt{\mu_i(1-\mu_i)}}{\sum_{j\in \mathbb{S}^*}\sqrt{\mu_j(1-\mu_j)}}\left(\frac{\sum_{j\in \mathbb{S}^*}\mu_j}{\lambda} - 1\right)\left(1 - \left(1 + \frac{2\delta}{\tilde{\mu}}\right)^4 \left(1 + \frac{\lvert \mathbb{S}^*\rvert \delta}{\sum_{j\in \mathbb{S}^*}\mu_j - \lambda}\right)\right)\\
        &\geq  -\frac{\delta}{\lambda} + \left(\frac{\sum_{j\in \mathbb{S}^*}\mu_j}{\lambda} - 1\right)\left(1 - \left(1 + 30\frac{\delta}{\tilde{\mu}}\right) \left(1 + \frac{\lvert \mathbb{S}^*\rvert \delta}{\sum_{j\in \mathbb{S}^*}\mu_j - \lambda}\right)\right)\\
        &\geq  -\frac{\delta}{\lambda} - \left(\frac{\sum_{j\in \mathbb{S}^*}\mu_j}{\lambda} - 1\right)\left(\frac{30\delta}{\tilde{\mu}} + \frac{\lvert \mathbb{S}^*\rvert \delta}{\sum_{j\in \mathbb{S}^*}\mu_j - \lambda} + \frac{30\delta^2 \lvert \mathbb{S}^*\rvert}{(\sum_{j\in \mathbb{S}^*}\mu_j - \lambda)\tilde{\mu}}\right)\\
        &\geq  -\delta\left(\frac{1}{\lambda} + \frac{30 \epsilon^*}{\lamda \tilde{\mu}} + \frac{16\lvert \mathbb{S}^*\rvert}{\lambda}\right)\\
        &\geq  -c_2\delta
    \end{align*}
    where $c_2 = \left(\frac{1}{\lambda} + \frac{30 \epsilon^*}{\lamda \tilde{\mu}} + \frac{16\lvert \mathbb{S}^*\rvert}{\lambda}\right)$. Hence, if $\delta \leq \Delta = \min \left\{\frac{\tilde{\mu}}{2}, \frac{\epsilon^*}{|\mathbb{S}^*|}, \frac{\epsilon^*}{2c\lambda}\right\}$ and $c = \max (c_1, c_2)$
    $$\lvert \hat{\mu}_i - \mu_i \rvert \leq  \delta,\>\> \forall i \implies \lvert \hat{p}_i - p_i^* \rvert \leq  \min\left\{c \delta, \frac{\epsilon^*}{2\lambda}\right\},\>\> \forall i$$
    \item
    \textit{Proof of lemma \ref{lm_conc_geoemtric}}\label{prf_lm_conc_geoemtric}
    \begin{align*}
        \left|\frac{\sum_i X_i}{n} - \frac{1}{\mu}\right| \leq x &\implies \frac{1}{\mu} - x \leq \frac{\sum_i X_i}{n} \leq \frac{1}{\mu} + x\\
        &\implies \frac{\mu}{1+xp}\leq \frac{n}{\sum_i X_i} \leq \frac{\mu}{1-xp}\\
        &\implies \frac{-xp^2}{1+xp}\leq \frac{n}{\sum_i X_i} - \mu \leq \frac{xp^2}{1-xp}\\
        &\implies -xp^2\leq \frac{n}{\sum_i X_i} - \mu \leq 2xp^2,\>\>\>\forall x \in [0, \frac{1}{2p}]\\
        &\implies \left|\frac{n}{\sum_i X_i} - \mu\right| \leq 2 x p^2\\
    \end{align*}
    Hence, 
    \begin{equation}\label{relation_p_mu_1}
        \left|\frac{\sum_i X_i}{n} - \frac{1}{\mu}\right| \leq x &\implies  \left|\frac{n}{\sum_i X_i} - \mu\right| \leq 2xp^2, \forall x \in \left[0, \frac{1}{2p}\right]
    \end{equation}
    Consider the following events
    \begin{equation*}
        \mathcal{G}_1(x) := \left|\frac{n}{\sum_i X_i} - \mu\right| \geq x
    \end{equation*}
    \begin{equation*}
        \mathcal{G}_2(x) := \left|\frac{\sum_i X_i}{n} - \frac{1}{\mu}\right| \geq x
    \end{equation*}
    Using \ref{relation_p_mu_1}, we get
    \begin{equation}\label{relation_p_mu_2}
        \probability\left(\mathcal{G}_1(x)\right)  \leq \probability\left(\mathcal{G}_2\left(\frac{x}{2p^2}\right)\right),\>\> \forall x\in [0, \mu]
    \end{equation}
    To bound the probability of $\mathcal{G}_1(t)$, we will in-turn bound the probability of $\mathcal{G}_2(t)$. Consider the 2 scenarios
    \begin{enumerate}
        \item \textit{Bounding the upper confidence interval}
            \begin{align*}
            \probability\left(\frac{\sum_i X_i}{n} \geq \frac{1}{\mu} + x\right) & \leq \left(\frac{\expectatione^{sX_1}}{e^{s(\frac{1}{\mu} + x)}}\right)^n,\>\>\>\> \forall s \geq 0\\
            &\leq \left(\frac{\expectatione^{sX_1}}{e^{s(\frac{1}{\mu} + x)}}\right)^n,\>\>\>\> \forall s \leq -\ln(1-\mu)\\
            &\leq \left(\frac{\frac{pe^s}{1-(1-\mu)e^s}}{e^{s(\frac{1}{\mu} + x)}}\right)^n\\
            &\leq \exp\left(n\left(\ln \mu +s - \ln(1-(1-\mu)e^s)- s\left(\frac{1}{\mu} + x\right)\right)\right)\\
        \end{align*}
        Now, define the function $f$ such that
        $$f(s) = \ln \mu +s - \ln(1-(1-\mu)e^s)- s\left(\frac{1}{\mu} + x\right)$$
        $$f'(s) = 1 +\frac{(1-\mu)e^s}{1-(1-\mu)e^s}- \left(\frac{1}{\mu} + x\right) = \frac{1}{1-(1-\mu)e^s}- \left(\frac{1}{\mu} + x\right)$$
        $$f''(s) = \frac{(1-\mu)e^s}{\left(1-(1-\mu)e^s\right)^2}\geq 0$$
        Hence, $f(s)$ is convex w.r.t $s$. This implies that the minima of the function is at the point where derivative is $0$. Thus
        \begin{align*}
             &\frac{1}{1-(1-\mu)e^{s^*}}- \left(\frac{1}{\mu} + x\right) =0\\
             \implies e^{s^*} &= \frac{1+\mu x-\mu}{1+\mu x-\mu-\mu^2x} \leq \frac{1}{1-\mu}
        \end{align*}
        Hence, 
        \begingroup
        \allowdisplaybreaks
        \begin{align*}
            f^* =& \ln \mu +s - \ln(1-(1-\mu)e^s)- s\left(\frac{1}{\mu} + x\right)\\
            =& \ln \left(1+\frac{px}{1-\mu}\right)- \left(\frac{1}{\mu} + x\right)\ln \left(1 + \frac{\mu^2x}{(1-\mu)(1+\mux)}\right)\\
            \overset{(a)}{\leq}& \frac{\mu x}{1-\mu} - \frac{1}{2}\left(\frac{\mu x}{1-\mu}\right)^2 + \frac{1}{2}\left(\frac{\mu x}{1-\mu}\right)^3 -\\
            &\left(\frac{1}{\mu} + x\right)\left(\frac{\mu^2x}{(1-\mu)(1+\mu x)}  -\frac{1}{2}\left(\frac{\mu^2x}{(1-\mu)(1+\mu x)}\right)^2\right)\\
            \leq& - \frac{1}{2}\left(\frac{\mu x}{1-\mu}\right)^2\left(1- \frac{\mu x}{1 - \mu} - \frac{\mu}{1 + \mu x}\right)\\
            \overset{(b)}{\leq}& - \frac{1}{2}\left(\frac{\mu x}{1-\mu}\right)^2\left(1- \frac{1-\mu}{2} - \mu\right)\\
            \leq& -\frac{\mu^2x^2}{4(1-\mu)}
        \end{align*}
        \endgroup
        where
        \begin{itemize}
            \item $(a)$ Used the fact $x - \frac{x^2}{2} \leq \ln (1 + x) \leq x - \frac{x^2}{2} + \frac{x^3}{2}$
            \item $(a)$ Used the fact $0 \leq x \leq \frac{1-\mu}{2\mu}$
        \end{itemize}
        Since, 
        $$\probability\left(\frac{\sum_i X_i}{n} \geq \frac{1}{\mu} + x\right) \leq \exp\left(n f(s)\right), \forall s \in \left[0, -\ln(1-\mu)\right]$$
        and $s^*$ lies in the interval $\left[0, -\ln(1-\mu)\right]$
        \begin{equation}\label{rel_upper_confidence}
            \probability\left(\frac{\sum_i X_i}{n} \geq \frac{1}{\mu} + x\right) \leq \exp\left(n f^*\right) = \exp\left(-\frac{\mu^2x^2}{4(1-\mu)}\right),\>\>\>\forall x\in \left[0, \frac{1-\mu}{2\mu}\right]
        \end{equation}
    \item \textit{Bounding the lower confidence interval}
        \begin{align*}
            \probability\left(\frac{\sum_i X_i}{n} \leq \frac{1}{\mu} - x\right) & \leq \left(\frac{\expectatione^{-sX_1}}{e^{-s(\frac{1}{\mu} - x)}}\right)^n,\>\> \forall s \geq 0\\
            &\leq \left(\frac{\expectatione^{-sX_1}}{e^{-s(\frac{1}{\mu} - x)}}\right)^n\\
            &\leq \left(\frac{\frac{pe^{-s}}{1-(1-\mu)e^{-s}}}{e^{-s(\frac{1}{\mu} - x)}}\right)^n\\
            &\leq \exp\left(n\left(\ln \mu -s - \ln(1-(1-\mu)e^{-s})+ s\left(\frac{1}{\mu} - x\right)\right)\right)\\
        \end{align*}
        Now define the function $g$ such that
        $$g(s) = \ln \mu -s - \ln(1-(1-\mu)e^{-s})+ s\left(\frac{1}{\mu} - x\right)$$
        $$g'(s) = -1 -\frac{(1-\mu)e^{-s}}{1-(1-\mu)e^{-s}}+ \left(\frac{1}{\mu} - x\right) = -\frac{1}{1-(1-\mu)e^{-s}}+ \left(\frac{1}{\mu} - x\right)$$
        $$g''(s) = \frac{(1-\mu)e^{-s}}{\left(1-(1-\mu)e^{-s}\right)^2}\geq 0$$
        Hence, $g(s)$ is convex w.r.t $s$. This implies that the minima of the function is at the point where derivative is $0$. Thus
        \begin{align*}
             &\frac{1}{1-(1-\mu)e^{-s^*}}- \left(\frac{1}{\mu} - x\right) =0\\
             \implies e^{-s^*} &= \frac{1-\mu x-\mu}{1-\mu x-\mu+\mu^2x} \leq 1
        \end{align*}
        To ensure that the minima is valid $e^{-s^*}\geq 0 \implies x\leq \frac{1-\mu}{\mu}$. Hence,  
        \begin{align*}
            g^* &= \ln \mu -s - \ln(1-(1-\mu)e^{-s})+ s\left(\frac{1}{\mu} - x\right)\\
            &= \ln \left(1-\frac{\mu x}{1-\mu}\right)- \left(\frac{1}{\mu} - x\right)\ln \left(1 - \frac{\mu^2x}{(1-\mu)(1-\mu x)}\right)\\
        \end{align*}
        Now, we want to argue that $\exists t_{g_-},c_{g_-} > 0$ such that $g(x)\leq -c_{g_-} x^2,\> \forall x \leq t_{g_-}$. Consider the function $h(x) = g(x) + c_{g_-}x^2$
        Now,
        \begin{align*}
            h(0) =& g(0) =0\\
            h'(x) =& g'(x) + 2c_{g_-}x\\
            =& \frac{\mu}{\mu x + \mu - 1} - \frac{1-\mu x}{\mu}\left[\frac{\mu}{\mu x + \mu - 1} - \frac{\mu^2-\mu}{1 - \mu - \mu x + \mu^2x}\right] + \\
            &\ln\left(\frac{1-\mu-\mu x}{1 - \mu - \mu x + \mu^2x}\right) + 2c_{g_-}x\\
            \implies h'(0) =& g'(0) = 0\\
            h''(x) =& -\frac{\mu^2}{(\mu x + \mu - 1)^2} - \frac{1-\mu x}{\mu}\left[-\frac{\mu^2}{(\mu x + \mu - 1)^2} + \frac{(\mu^2-\mu)^2}{(1 - \mu - \mu x + \mu^2 x)^2}\right] + \\
            & 2\left[\frac{\mu}{\mu x + \mu - 1} - \frac{\mu^2-\mu}{1 - \mu - \mu x + \mu^2 x}\right] + 2c_g\\
            \implies h''(0) =& -\frac{\mu^2}{1-\mu} + 2c_{g_-}
        \end{align*}
        Since , $h(0) = h'(0) = 0$ and $\exists c_{g_-} \leq \frac{\mu^2}{2(1-\mu)}$ such that $h''(0) < 0 \implies \exists t_{g_-} \geq 0$ s.t. $g(x) \leq -c_{g_-}x^2,\>\forall x\leq t_{g_-}$.
        Since, 
        $$\probability\left(\frac{\sum_i X_i}{n} \leq \frac{1}{\mu} - x\right) \leq \exp\left(n g(s)\right), \forall s \geq 0$$
        and $s^*\geq 0$, if $x \leq \frac{1-\mu}{\mu}$
        \begin{equation}\label{rel_lower_confidence}
            \probability\left(\frac{\sum_i X_i}{n} \leq \frac{1}{\mu} - x\right) \leq \exp\left(n g^*\right) \leq \exp\left(-nc_{g_-} x^2\right),\>\>\>\forall x\in \left[0,\min\left\{\frac{1-\mu}{\mu}, t_{g_-}\right\}\right]
        \end{equation}
    \end{enumerate}
    Using \ref{rel_upper_confidence} and \ref{rel_lower_confidence}, we get  
    \begin{equation}
        \probability\left(\left|\frac{\sum_i X_i}{n} - \frac{1}{\mu}\right| \geq x\right) \leq  \exp\left(-n c_g'x^2\right),\>\> \forall x \in [0, t_g']
    \end{equation}
    where $c_g' = \min\left\{\frac{\mu^2}{4(1-\mu)}, c_{g_-} \right\}, t_g'=\min\left\{\frac{1-\mu}{2\mu}, t_{g_-}, \frac{1}{2\mu}\right\}$. Finally using \ref{relation_p_mu_2}, we get
    \begin{equation}
        \probability\left(\left|\frac{n}{\sum_i X_i} - \mu\right| \geq x\right) \leq  \exp\left(-n c_gt^2\right),\>\> \forall x \in [0, t_g]
    \end{equation}
    where $c_g = \min\left\{\frac{c_g'}{4\mu^4}, 1\right\}, t_g = 2\mu^2t_g'$
    \item \textit{Proof of Lemma \ref{lm_p_wt}}\label{prf_lm_p_wt}\\
    We will prove it for $\tau = w_1(t)$ and use union bound for $\tau \geq w_1(t)$.
    \begin{align*}
        \probability\left(\left|\hat{\mu}_i(\tau) - \mu_i\right|> \Delta_0\right) &= \probability\left(\left|\hat{\mu}_i(\tau) - \mu_i\right|> \Delta_0, \sum_{l=1}^{\tau} \departure_i(l) < n_0\right) + \sum_{n=n_0}^{\infty}\probability\left(\left|\hat{\mu}_i(\tau) - \mu_i\right|> \Delta_0, \sum_{l=1}^{\tau} \departure_i(l) = n\right)\\
        &\leq \probability\left(\sum_{l=1}^{\tau} \departure_i(l) < n_0\right) + \sum_{n=n_0}^{\infty}\probability\left(\left|\hat{\mu}_i^{(n)} - \mu_i\right|> \Delta_0, \sum_{l=1}^{\tau} \departure_i(l) = n\right)\\
        &\leq \probability\left(\sum_{l=1}^{\tau} \departure_i(l) < n_0\right) + \sum_{n=n_0}^{\infty}\probability\left(\left|\hat{\mu}_i^{(n)} - \mu_i\right|> \Delta_0, \right)\\
        &\leq \probability\left( \sum_{l=1}^{\tau}\departure_i(l) < n_0 \Big| \sum_{l=1}^{\tau/2}\arrival_i(l) \geq n_0\right) + \probability \left(\sum_{l=1}^{\tau/2} \arrival_i(l) < n_0\right) + \sum_{n=n_0}^{\infty}\exp\left( -n c_g\Delta_0^2 \right)\\
        &\leq \underbrace{\probability\left( \sum_{l=1}^{\tau}\departure_i(l) < n_0 \Big| \sum_{l=1}^{\tau/2}\arrival_i(l) \geq n_0\right)}_{T_1} + \underbrace{\probability \left(\sum_{l=1}^{\tau/2} \arrival_i(l) < n_0\right)}_{T_2} +  \underbrace{\frac{\exp\left( -n_0 c_g\Delta_0^2 \right)}{1 - \exp\left( -c_g\Delta_0^2 \right)}}_{T_3}
    \end{align*}
    where $\hat{\mu}_i^{(n)}$ is the estimate of $\mu_i$ using $n$ independent samples of i.i.d. geometric random variable with parameter $\mu_i$. Take $n_0 = \frac{4\ln t}{c_g \Delta_0^2}$. Since the probability of exploration at each time $t$ is $\frac{K\lambda\ln t}{t}$, we have
    $$\probability\left(\explore_i(t) = 1\right) = \frac{\lambda\ln t}{t},\> \forall t$$
    Hence, 
    $$\expectation\left(\sum_{l=1}^{\tau/2}\explore_i(l)\right) = \frac{1}{2}\lambda\ln^2\left(\frac{\tau}{2}\right)= \frac{8\ln t}{c_g \Delta_0^2}$$
    Bounding $T_1$,we get 
    \begin{align*}
        \probability\left(\sum_{l=1}^{\tau/2}\arrival_i(l) <\frac{4\ln t}{c_g \Delta_0^2}\right) & \leq \probability\left(\sum_{l=1}^{\tau/2}\explore_i(l) \leq \frac{4\ln t}{c_g \Delta_0^2}\right)\\
        & \leq \probability\left(\sum_{l=1}^{\tau/2}\explore_i(l)  \leq \left(1-\frac{1}{2}\right)\expectation\left(\sum_{l=1}^{\tau/2}\explore_i(l) \right)\right)\\
        &\leq exp\left(-\frac{1}{8}\expectation\left(\sum_{l=1}^{\tau/2}\explore_i(l) \right)\right)\\
        &\leq exp\left(-\frac{4\ln t}{8\Delta_0^2 c_g}\right)\\
        &\overset{(a)}{\leq} \frac{1}{t^{8}}
    \end{align*}
    where, $(a)$ uses the fact that $\Delta_0 \leq \frac{\tilde{\mu}}{2} \leq \frac{1}{4}$ and $c_g \leq 1$. Bounding $T_2$,we get
    \begingroup\allowdisplaybreaks
    \begin{align*}
        &\probability\left( \sum_{l=1}^{\tau}\departure_i(l)  < \frac{4\ln t}{c_g \Delta_0^2} \Big| \sum_{l=1}^{\tau/2}\arrival_i(l) > \frac{4\ln t}{c_g \Delta_0^2}\right) \\
        \leq& \probability\left(\sum_{l=1}^{\tau/2}\departure_i(l)=0\right)\probability\left( \sum_{l=1}^{\tau}\departure_i(l) < \frac{4\ln t}{c_g \Delta_0^2} \Big| \sum_{l=1}^{\tau/2}\arrival_i(l) > \frac{4\ln t}{c_g \Delta_0^2}, \sum_{l=1}^{\tau/2}\departure_i(l)=0\right) + \\
        & \probability\left(\sum_{l=1}^{\tau/2}\departure_i(l)\neq 0\right)\probability\left( \sum_{l=1}^{\tau}\departure_i(l) < \frac{4\ln t}{c_g \Delta_0^2} \Big| \sum_{l=1}^{\tau/2}\arrival_i(l) > \frac{4\ln t}{c_g \Delta_0^2}, \sum_{l=1}^{\tau/2}\departure_i(l)\neq 0\right)\\
        \overset{(a)}{\leq}& \probability\left( \sum_{l=1}^{\tau}\departure_i(l) < \frac{4\ln t}{c_g \Delta_0^2} \Big| \sum_{l=1}^{\tau/2}\arrival_i(l) > \frac{4\ln t}{c_g \Delta_0^2}, \sum_{l=1}^{\tau/2}\departure_i(l)= 0\right)\\
        =& \probability\left( \sum_{l=\tau/2}^{\tau}\service_i(l) < \frac{4\ln t}{c_g \Delta_0^2}\right)\\
        \overset{(b)}{\leq}& \probability\left( \sum_{l=1}^{\tau/2}\explore_i(l) < \frac{4\ln t}{c_g \Delta_0^2}\right)\\
        \leq& \frac{1}{t^{8}}
    \end{align*}
    \endgroup
    where,
    \begin{itemize}
        \item $(a)$ uses the fact that the second term is strictly smaller than the first term.
        \item $(b)$ uses the fact that that mean of $\service_i(l)$ is strictly larger than that of $\explore_i(l)$ and we can use coupling argument to show rest of the argument.
    \end{itemize}
    Using the above relation we have,
    \begin{equation}
        \probability\left(\left|\hat{\mu}_i(\tau) - \mu_i\right|> \Delta_0\right) = \leq \frac{2}{t^8} + \frac{k_2}{t^4},\\
    \end{equation}
    where $k_2 = \frac{1}{1 - \exp\left( -c_g\Delta_0^2 \right)}$. 
    % \\\\\
    % Consider the following events.
    % \begin{equation}
    %     \mathcal{E}_{111} := |\hat{\mu}_i(\tau) - \mu_i| < \Delta_0.
    % \end{equation}
    % \begin{equation}
    %     \mathcal{E}_{112} := \sum_{l = 1}^{\frac{\tau}{2}} A_i(l) > \frac{4\ln t}{c_g \Delta_0^2}.
    % \end{equation}
    % \begin{equation}
    %     \mathcal{E}_{113} := |\hat{\mu}_i^{(n)} - \mu_i| < \Delta_0,\> n = \frac{4\ln t}{c_g \Delta_0^2},
    % \end{equation}
    % where $\hat{\mu}_i^{(n)}$ is the estimate of $\mu_i$ using $n$ independent samples of i.i.d. geometric random variable with parameter $\mu_i$.
    % \begin{equation}
    %     \mathcal{E}_{114} := \mbox{Time to depart $n$ jobs from server $i$} \leq \frac{\tau}{2}.
    % \end{equation}
    % Now 
    % \begin{equation}
    %     \mathcal{E}_{111} =\mathcal{E}_{112}\cap \mathcal{E}_{113} \cap\mathcal{E}_{114}
    % \end{equation}
    % We will now bound each of the term as follows
    % \begin{itemize}
    %     \item  \textit{Bounding probability of event $\mathcal{E}_{112}$} - 
    %     $$\probability\left(\explore_i(t) = 1\right) = \frac{\lambda\ln t}{t},\> \forall t$$
    %     Hence, 
    %     $$\expectation\left(\sum_{l=1}^{\tau/2}\explore_i(l)\right) = \frac{1}{2}\lambda\ln^2\left(\frac{\tau}{2}\right)= \frac{8\ln t}{c_g \Delta_0^2}$$
    %     Hence, 
    %     \begin{align*}
    %         \probability\left(\mathcal{E}_{112}^c\right) & \leq \probability\left(\sum_{l=1}^{\tau/2}\explore_i(l) \leq \frac{4\ln t}{c_g \Delta_0^2}\right)\\
    %         & \leq \probability\left(\sum_{l=1}^{\tau/2}\explore_i(l)  \leq \left(1-\frac{1}{2}\right)\expectation\left(\sum_{l=1}^{\tau/2}\explore_i(l) \right)\right)\\
    %         &\leq exp\left(-\frac{1}{8}\expectation\left(\sum_{l=1}^{\tau/2}\explore_i(l) \right)\right)\\
    %         &\leq exp\left(-\frac{4\ln t}{8\Delta_0^2 c_g}\right)\\
    %         &\overset{(a)}{\leq} \frac{1}{t^{8}}
    %     \end{align*}
    %     where, $(a)$ uses the fact that $\Delta_0 \leq \frac{\tilde{\mu}}{2} \leq \frac{1}{4}$ and $c_g \leq 1$.
    %     \item \textit{Bounding probability of event $\mathcal{E}_{113}$} - \\
    %     For at-least $\frac{4\ln t}{c_g \Delta_0^2}$ departures from the server $i$, the estimate $\hat{\mu}_i$ can be bounded using lemma \ref{lm_conc_geoemtric} as
    %     \begin{align*}
    %         \probability\left(|\hat{\mu}_i - \mu_i| > \Delta_0 \right) &\leq \exp\left(-c_g \frac{4\ln t}{c_g \Delta_0^2} \Delta_0^2\right)\\
    %         &\leq \exp\left(-4\ln t\right)\\
    %         &\leq \frac{1}{t^4}
    %     \end{align*}
    %     \item \textit{Bounding probability of event $\mathcal{E}_{114}$} - \\
    %     Let $X_1, X_2, \cdots, X_n$ be the time taken by the jobs respectively. Now, 
    %     \begin{align*}
    %         |\hat{\mu}_i^{(n)} - \mu_i| &\leq \Delta_0\\
    %         \implies |\hat{\mu}_i^{(n)}  - \mu_i| & \overset{(a)}{\leq} \frac{\mu_i}{2}\\
    %         \implies \hat{\mu}_i^{(n)} &\geq \frac{\mu_i}{2}\\
    %         \implies \sum_i X_i &\leq \frac{8\ln t}{\mu_i c_g \Delta_0^2}\\
    %         \implies \sum_i X_i &\overset{(b)}{\leq} \frac{\tau}{2}\\
    %         \implies \mbox{Time taken to depart $n$ jobs} &\leq \frac{\tau}{2}\\
    %         \implies \mathcal{E}_{113} &\subseteq \mathcal{E}_{114}
    %     \end{align*}
    %     where $(a), (b)$ follows from the definition of $\Delta_0, t_0$
    % \end{itemize}
    % This gives, 
    % \begin{equation}
    %     \probability\left(|\hat{\mu}_i(\tau) - \mu_i| > \Delta_0 \right) = \probability\left(\mathcal{E}_{111}^c\right) \leq \probability\left(\mathcal{E}_{112}^c\right) + \probability\left(\mathcal{E}_{113}^c\right) +  \probability\left(\mathcal{E}_{114}^c\right) \leq \frac{2}{t^4} + \frac{1}{t^8}
    % \end{equation}
    % For any event $A, B$,
    % \begin{equation}\label{eqn_prb_2_events}
    %     \probability(A) = \probability(B)\probability(A|B) + \probability(B^c)\probability(A|B^c) \leq  \probability(A|B) + \probability(B^c)
    % \end{equation}
    % Using the equation,
    % \begingroup
    % \allowdisplaybreaks
    % \begin{align*}
    %     \probability\left(|\hat{\mu}_i(\tau) - \mu_i| \geq \Delta_0\right) \leq& \probability\left(|\hat{\mu}_i(\tau) - \mu_i| \geq \Delta_0 \Big| \sum_{l=1}^{\tau}\departure_i(l) \geq \frac{4\ln t}{c_g \Delta_0^2}\right) + \probability\left( \sum_{l=1}^{\tau}\departure_i(l) \leq \frac{4\ln t}{c_g \Delta_0^2}\right)\\
    %     \leq& \underbrace{\probability\left(|\hat{\mu}_i(\tau) - \mu_i| \geq \Delta_0 \Big| \sum_{l=1}^{\tau}\departure_i(l) \geq \frac{4\ln t}{c_g \Delta_0^2}\right)}_{T_1} +\\
    %     &\underbrace{\probability\left( \sum_{l=1}^{\tau}\departure_i(l) \leq \frac{4\ln t}{c_g \Delta_0^2} \Big| \sum_{l=1}^{\tau/2}\arrival_i(l) \geq \frac{4\ln t}{c_g \Delta_0^2}\right)}_{T_2} + \underbrace{\probability \left(\sum_{l=1}^{\tau/2} \arrival_i(l) \leq \frac{4\ln t}{c_g \Delta_0^2}\right)}_{T_3}\\
    % \end{align*}
    % \endgroup
    % Since the probability of exploration at each time $t$ is $\frac{K\lambda\ln t}{t}$, we have
    % $$\probability\left(\explore_i(t) = 1\right) = \frac{\lambda\ln t}{t},\> \forall t$$
    % Hence, 
    % $$\expectation\left(\sum_{l=1}^{\tau/2}\explore_i(l)\right) = \frac{1}{2}\lambda\ln^2\left(\frac{\tau}{2}\right)= \frac{8\ln t}{c_g \Delta_0^2}$$
    % Bounding $T_3$,we get 
    % \begin{align*}
    %     \probability\left(\sum_{l=1}^{\tau/2}\arrival_i(l) <\frac{4\ln t}{c_g \Delta_0^2}\right) & \leq \probability\left(\sum_{l=1}^{\tau/2}\explore_i(l) \leq \frac{4\ln t}{c_g \Delta_0^2}\right)\\
    %     & \leq \probability\left(\sum_{l=1}^{\tau/2}\explore_i(l)  \leq \left(1-\frac{1}{2}\right)\expectation\left(\sum_{l=1}^{\tau/2}\explore_i(l) \right)\right)\\
    %     &\leq exp\left(-\frac{1}{8}\expectation\left(\sum_{l=1}^{\tau/2}\explore_i(l) \right)\right)\\
    %     &\leq exp\left(-\frac{4\ln t}{8\Delta_0^2 c_g}\right)\\
    %     &\overset{(a)}{\leq} \frac{1}{t^{8}}
    % \end{align*}
    % where, $(a)$ uses the fact that $\Delta_0 \leq \frac{\tilde{\mu}}{2} \leq \frac{1}{4}$ and $c_g \leq 1$. Bounding $T_2$,we get
    % \begingroup\allowdisplaybreaks
    % \begin{align*}
    %     &\probability\left( \sum_{l=1}^{\tau}\departure_i(l)  < \frac{4\ln t}{c_g \Delta_0^2} \Big| \sum_{l=1}^{\tau/2}\arrival_i(l) > \frac{4\ln t}{c_g \Delta_0^2}\right) \\
    %     \leq& \probability\left(\sum_{l=1}^{\tau/2}\departure_i(l)=0\right)\probability\left( \sum_{l=1}^{\tau}\departure_i(l) < \frac{4\ln t}{c_g \Delta_0^2} \Big| \sum_{l=1}^{\tau/2}\arrival_i(l) > \frac{4\ln t}{c_g \Delta_0^2}, \sum_{l=1}^{\tau/2}\departure_i(l)=0\right) + \\
    %     & \probability\left(\sum_{l=1}^{\tau/2}\departure_i(l)\neq 0\right)\probability\left( \sum_{l=1}^{\tau}\departure_i(l) < \frac{4\ln t}{c_g \Delta_0^2} \Big| \sum_{l=1}^{\tau/2}\arrival_i(l) > \frac{4\ln t}{c_g \Delta_0^2}, \sum_{l=1}^{\tau/2}\departure_i(l)\neq 0\right)\\
    %     \overset{(a)}{\leq}& \probability\left( \sum_{l=1}^{\tau}\departure_i(l) < \frac{4\ln t}{c_g \Delta_0^2} \Big| \sum_{l=1}^{\tau/2}\arrival_i(l) > \frac{4\ln t}{c_g \Delta_0^2}, \sum_{l=1}^{\tau/2}\departure_i(l)= 0\right)\\
    %     =& \probability\left( \sum_{l=\tau/2}^{\tau}\service_i(l) < \frac{4\ln t}{c_g \Delta_0^2}\right)\\
    %     \overset{(b)}{\leq}& \probability\left( \sum_{l=1}^{\tau/2}\explore_i(l) < \frac{4\ln t}{c_g \Delta_0^2}\right)\\
    %     \leq& \frac{1}{t^{8}}
    % \end{align*}
    % \endgroup
    % where,
    % \begin{itemize}
    %     \item $(a)$ uses the fact that the second term is strictly smaller than the first term.
    %     \item $(b)$ uses the fact that that mean of $\service_i(l)$ is strictly larger than that of $\explore_i(l)$ and we can use coupling argument to show rest of the argument.
    % \end{itemize}
    % Finally using lemma \ref{lm_conc_geoemtric} and bounding $T_1$, we get
    % \begin{align*}
    %     \probability\left(|\hat{\mu}_i(\tau) - \mu_i| > \Delta_0 \Big| \sum_{l=1}^{\tau}\departure_i(l) > \frac{4\ln t}{c_g \Delta_0^2}\right) &\leq \exp\left(-c_g \frac{4\ln t}{c_g \Delta_0^2} \Delta_0^2\right)\\
    %     &\leq \exp\left(-4\ln t\right)\\
    %     &\leq \frac{1}{t^4}
    % \end{align*}
    Union bounding for $\tau \in \left[w(t), t\right]$ and for all $i$, we get 
    \begin{equation}\label{rel_mu_wt}
        \probability\left(|\hat{\mu}_i(\tau) - \mu_i| \geq \Delta_0\right) \leq \numofserver\left(\frac{2}{t^{7}} + \frac{k_2}{t^3}\right),\> \forall i,\mbox{for any }\tau \in\left[w(t), t\right]
    \end{equation}
    Now, $\forall i, \forall \tau\ in \left[w(t), t\right],\> |\hat{\mu}_i(\tau) - \mu_i| \leq \Delta_0$ implies that
    \begin{enumerate}
        \item $|\hat{\mu}_i(\tau) - \mu_i| \leq \Delta_{support} \implies \support(\tau) = \support^*\implies \mathcal{E}_{11} \mbox{ is true}$
        \item $|\hat{\mu}_i(\tau) - \mu_i|\leq \min\left\{\Delta, \frac{p_{min}^*}{2c}\right\} \implies \left|\hat{p}_i(\tau) - p_i^* \right|\leq \frac{p_i^*}{2}\implies \frac{p_i^*}{2} \leq \hat{p}_i(\tau)\leq \frac{3p_i^*}{2} \implies \mathcal{E}_{12} \mbox{ is true}$
        \item $|\hat{\mu}_i(\tau) - \mu_i|\leq \Delta \implies \lambda\left|\hat{p}_i(\tau) - p_i^* \right|\leq \frac{\epsilon_i^*}{4}$\\
        Now, 
        \begin{align*}
            \expectation\left(\arrival_i(\tau)\right) &\leq \lambda\left(\frac{\ln \tau}{\tau} + \hat{p}_i(\tau)\right)\\
            &\leq \frac{\lambda\ln \tau}{\tau} + \lambda\hat{p}_i(\tau) - \lambda p_i^* + \lambda p_i^*\\
            &\leq \frac{\lambda\ln \tau}{\tau} + \mu_i - \frac{3\epsilon_i}{4}\\
            &\leq \mu_i - \frac{\epsilon_i}{2}
        \end{align*}
        The last step is true if $\frac{\lambda\ln (w(\tau))}{(w(\tau))} \leq \frac{\lambda}{\sqrt{w(\tau)}}\leq \frac{\lambda \sqrt{\epsilon_i}}{\sqrt{48 \ln \tau}} \leq \frac{\epsilon_i}{4} \implies \tau \geq \exp\left(\frac{\lambda}{48\epsilon_i^2}\right)$, which is true
    \end{enumerate}
    Hence, 
    \begin{equation}\label{rel_lm_p_wt}
        \probability\left(\eventone^c\right) \leq \numofserver\left(\frac{2}{t^{7}} + \frac{k_2}{t^3}\right)
    \end{equation}
    \item \textit{Proof of Lemma \ref{lm_bound_q_length}}\label{prf_lm_bound_q_length}\\
    \begin{equation}\label{rel_bound_q}
        \probability\left(\queue_i(\tau)\geq 2w(t)\right)  \leq \probability\left(\queue_i(\tau)\geq 2w(t)\Big | \eventone\right) + \probability\left(\eventone^c\right)
    \end{equation}
    Notice, for all $\tau \geq w(t)$
    \begingroup
    \allowdisplaybreaks
    \begin{align*}
        \queue_i(\tau) \geq 2w(t) &= \sum_{l=1}^{\tau}\left[ \arrival_i(l) - \departure_i(l)\right]\\
        &= \sum_{l=1}^{w(t)}\left[ \arrival_i(l) - \departure_i(l)\right]
         + \sum_{w(t)}^{\tau}\left[ \arrival_i(l) - \departure_i(l)\right]\\
         &\leq w(t) + \sum_{w(t)}^{\tau} \left[ \arrival_i(l) - \departure_i(l)\right]
    \end{align*}
    \endgroup
    Now,
    \begin{align}\label{rel_queue_for_all_t}
        & \queue_i(\tau) \geq 2w(t) \\
        \implies &\sum_{l=w(t)}^{\tau}\left[ \arrival_i(l) - \departure_i(l)\right]\geq w(t) \\
        \implies& \exists l_1, l_2\in (w(t), t) \mbox{ such that } (l_2 - l_1) \geq w(t),  \queue_i^{(l)}>0,\> \forall l \in [l_1, l_2],\sum_{l=l_1}^{l_2}\left[ \arrival_i(l) - \departure_i(l)\right]\geq w(t)\\
        \implies& \exists l_1, l_2\in (w(t), t) \mbox{ such that } (l_2 - l_1) \geq w(t),\sum_{l=l_1}^{l_2}\left[ \arrival_i(l) - \service_i(l)\right]\geq w(t)
    \end{align}
    Also, notice that
    \begin{equation}{\label{rel_lnwt_wt}}
        t \geq \exp\left(\frac{\lambda c_g \Delta_0^2}{16} \ln^2\left(8\left(\frac{\lambda}{\epsilon_i^*}\right)^2\right)\right)\implies w(t) \geq 16\left(\frac{\lambda}{\epsilon_i^*}\right)^2 \implies \frac{\ln w(t)}{w(t)} \leq \frac{1}{\sqrt{w(t)}} \leq \frac{\epsilon_i^*}{4\lambda}
    \end{equation}
    Hence,  
    \begin{align*}
        \expectation\left(\sum_{l=l_1}^{l_2} \left[ \arrival_i (l) - \service_i(l)\right]\Big| \eventone\right) &\leq -\frac{\epsilon_i^*}{4}\left(l_2 - l_1\right)
    \end{align*}
    implying 
    \begin{align*}
        \probability\left(\queue_i^{(\tau)}\geq 2w(t)\Big| \eventone\right) \leq& 
        \probability\left(\sum_{l=l_1}^{l_2} \left[ \arrival_i (l) - \service_i(l) \right]\geq w(t)\Big | \eventone\right) \\
        \overset{(a)}{\leq}& \exp\left(-\frac{\left(\frac{\epsilon_i^*}{4}\left(l_2 - l_1\right) + w(t)\right)^2}{4(l_2-l_1)}\right)\\
        \overset{(b)}{\leq}& \exp \left(-\frac{\epsilon_i^* w(t)}{8}\right)\\
        \overset{(c)}{\leq}& \frac{1}{t^6}
    \end{align*}
    where
    \begin{itemize}
        \item $(a)$ - Used Hoeffding's inequality
        \item $(b)$ - Used the inequality $AM\geq GM$ in the numerator
        \item $(c)$ - Used the definition of $t_0$
    \end{itemize}
    Taking an union bound $\forall l_1, l_2, \forall i$ and using equation \ref{rel_bound_q}, and lemma \ref{lm_p_wt}, we get,
    \begin{equation}
        \probability\left(\queue_i(\tau)\geq 2w(t)\right) \leq \numofserver \left( \frac{1}{t^4} + \frac{2}{t^{7}} + \frac{k_2}{t^3}\right), \>\> \forall \tau\in \left[w(t), t\right].
    \end{equation}
    \item \textit{Proof of Lemma \ref{lm_bound_busy_period_1}} \label{prf_lm_bound_busy_period_1}\\
    Given $\eventone$ and $\eventtwo$, $t_1 = t - v_i(t)-\frac{16}{3}w(t), t_2 = t-v_i(t)$ for any server $i$,
    \begin{align*}
        B_i(t - v_u(t))) \geq \frac{16w(t)}{3\epsilon_i} &\implies \sum_{l=t_1}^{t_2} \left[ \departure_i(l) - \arrival_i (l)\right] \leq 2w(t), \queue_i(\tau) > 0, \forall \tau\in [t_1, t_2]\\
        &\implies \sum_{l=t_1}^{t_2} \left[ \service_i(l) - \arrival_i (l)\right] \leq 2w(t)\\
    \end{align*}
    Hence, 
    \begin{equation}\label{rel_sec_busy_period}
        \probability\left(\eventthree^c\right) \leq \probability\left(\eventthree^c\Big| \eventone, \eventtwo\right) + \probability\left(\eventone^c\right) + \probability\left(\eventtwo^c\right) 
    \end{equation}
    Now, 
    \begin{align*}
        \expectation\left(\sum_{l=t_1}^{t_2} \left[ \service_i(l) - \arrival_i (l)\right]\Big| \eventone, \eventtwo\right) &\geq \frac{\epsilon_i^*}{2}\left(t_2 - t_1\right) \geq \frac{8}{3} w(t)
    \end{align*}
    implying 
    \begin{align*}
        \probability\left(\eventthree^c\Big| \eventone, \eventtwo\right) &\leq \probability\left(\sum_{l=t_1}^{t_2} \left[ \service_i(l) - \arrival_i (l) \right]\leq 2w(t)\Big |  \eventone, \eventtwo\right)\\
        &\leq \exp \left(-\frac{2w(t)}{9}\right)\\
        &\overset{(a)}{\leq} \exp\left(-4\ln t\right)
        \leq \frac{1}{t^4}
    \end{align*}
    Taking union bound $\forall i$ and using equation \ref{rel_sec_busy_period}, we have,
    \begin{equation}
        \probability\left(\eventthree^c\right) \leq  \numofserver\left(\frac{4}{t^{7}} + \frac{2k_2}{t^3} + \frac{2}{t^4}\right)
    \end{equation}
    \item \textit{Proof of Lemma \ref{lm_tighter_queue_length}}\label{prf_lm_tighter_queue_length}\\
    Define $r(t) = t - v_i(t)$.
    \begin{equation}
        \queue_i(r(t)) = \sum_{l = r(t) - B_i(r(t))}^{r(t)} \explore_i(l) + \exploit_i(l) - \service_i(l)
    \end{equation}
    Consider the following events,
    \begin{enumerate}
        \item $\mathcal{E}_{41} := \sum_{l = r(t) - B_i(r(t))}^{r(t)} \explore_i(l) \leq 5 \max\left\{\ln t, \frac{1}{2}\left(\ln^2(r(t)) - \ln^2(r(t) - B_i(r(t)))\right)\right\}$
        \item $\mathcal{E}_{42} := \sum_{l = r(t) - B_i(r(t))}^{r(t)} \left[\exploit_i(l) - \service_i(l)\right] \leq \frac{16}{\epsilon^*} \ln t$
    \end{enumerate}
    For the event $\mathcal{E}_{61}$, we will use the following inequality, 
    \begin{equation}\label{rel_prob_explore}
        \probability\left(\sum_{l=t_1}^{t_2} \explore_i(l) \geq 5\max\left\{\ln t, \frac{1}{2}\log^2(t_2) - \frac{1}{2}\ln^2(t_1)\right\}\right)\leq \frac{1}{t^4}
    \end{equation}
    \Weina{You need to specify the for what values of $t_1$ and $t_2$ this is true.  Do they need to be both smaller than $t$?}
    for any $t$ and $t_1<t_2$. If $\expectation\left(\sum_{l=t_1}^{t_2} \explore_i(l)\right) \geq \ln t$, we can use the chernoff bound with $\delta = 4$
    \begin{equation}
        \probability\left(Y \geq (1+\delta)\expectation Y \right) \leq \left(\frac{e^\delta}{(1+\delta)^{1+\delta}}\right)^{\expectation Y}
    \end{equation}
    If, $\expectation\left(\sum_{l=t_1}^{t_2} \explore_i(l)\right) \geq \ln t$, consider another random variable $Y'$ which stochastically dominates $\explore_i(l)$ and has mean $\ln t$. Now, 
    \begin{equation}
        \probability\left(Y' \geq 5\ln t\right) \leq \probability\left(Y \geq 5\ln t\right) \leq \frac{1}{t^4}
    \end{equation}
    \Weina{Where is $Y'$ being used?  What is $Y$ in your problem and how is the Chernoff bound used?  How is this condition on $\expectation\left(\sum_{l=t_1}^{t_2} \explore_i(l)\right)$ justified?}
    Now, 
    \begin{equation}
        5 \max\left\{\ln t, \frac{1}{2}\left(\ln^2(r(t)) - \ln^2(r(t) - B_i(r(t)))\right)\right\} &\leq 5 \ln t + \frac{5}{2}\left(\ln^2(r(t)) - \ln^2(r(t) - B_i(r(t)))\right)\\
    \end{equation}
    Also, for any $t_1, t_2 \in [\frac{t}{2}, t]$
    \begin{equation}\label{rel_explore_t1_t2}
        \frac{1}{2}\left(\ln^2 t_2 - \ln^2 t_1\right) \leq \frac{(t_2 - t_1)\ln t_1}{t_1} \leq \frac{2(t_2 - t_1)\ln t}{t}
    \end{equation}
    Using the above equation, we can show that
    \Weina{This needs explanation.  I cannot see how to connect these arguments together.}
    \begin{equation}
        \eventfour \supseteq \mathcal{E}_{61} \cap \mathcal{E}_{62}
    \end{equation}
    \begin{equation}
        \probability\left(\eventfour^c\right) \leq \probability\left(\mathcal{E}_{41}^c\right\Big| \eventone, \eventthree) + \probability\left(\mathcal{E}_{42}^c\Big| \eventone, \eventthree\right) + \probability\left(\eventone^c\right) + \probability\left(\eventthree^c\right) 
    \end{equation}
    From equation \ref{rel_prob_explore} we know that, for any $i$
    \begin{equation}\label{rel_inter_lemma}
        \probability\left(\sum_{l = r(t) - B_i(r(t))}^{r(t)} \explore_i(l) \geq 5 \max\left\{\ln t, \frac{1}{2}\left(\ln^2(r(t)) - \ln^2(r(t) - B_i(r(t)))\right)\right\}\right) \leq \frac{1}{t^4}
    \end{equation}
    Similarly, for any $i$,  
    \begingroup
    \allowdisplaybreaks
    \begin{align*}
        &\probability\left(\sum_{l = r(t) - B_i(r(t))}^{r(t)} \exploit_i(l) - \service_i(l) \geq \frac{16}{\epsilon^*} \ln t \Big| B_i(r(t)) \geq \frac{16}{\epsilon^*} \ln t\right)\\
        \leq& \probability\left(\sum_{l = r(t) - B_i(r(t))}^{r(t)} \arrival_i(l) - \service_i(l) \geq 0\Big| B_i(r(t)) \geq \frac{16}{\epsilon^*} \ln t\right)\\
        \leq& \exp\left(-\frac{1}{2}\expectation\left(\sum_{l = r(t) - B_i(r(t))}^{r(t)} \arrival_i(l) - \service_i(l)\right)\right) \\
        \leq& \exp\left( -\frac{\epsilon_i^*}{4}\frac{16}{\epsilon^*}\ln t\right) \\
        \leq& \frac{1}{t^4}
    \end{align*}
    \endgroup
    Taking an union bound over all $i$ and using equation \ref{rel_inter_lemma} completes the proof.
    \item \textit{Proof of Lemma \ref{lm_final_busy_period}}\label{prf_lm_final_busy_period}
    \begin{equation}\label{rel_final_busy_period}
        \probability\left(\eventfive^c\right) \leq \probability\left(\eventfive^c\right\Big| \eventone, \eventfour) +  \probability\left(\eventone^c\right) +   \probability\left(\eventfour^c\right)
    \end{equation}
    Similar to the proof of lemma $\ref{lm_bound_busy_period_1}$, we can show that 
    \begin{equation}
        B_i(t) \geq \frac{96 \ln t}{\epsilon_i^2}, \queue_i(t - v_i(t)) \leq \frac{32\ln t}{\epsilon_i}, \queue_i(\tau)\geq 0, \forall \tau \in \left[r(t), t\right] \implies \sum_{l = t - v_i(t)}^{t} \left[\service_i(l) - \arrival_i(l)\right] \leq \frac{32\ln t}{\epsilon_i}
    \end{equation}
    \begin{align*}
        \expectation\left(\sum_{l = t - v_i(t)}^{t} \left[\service_i(l) - \arrival_i(l)\right]\Big| \eventone, \eventfour \right) \geq \frac{\epsilon_i^*}{2}v_i(t) \geq \frac{48 \ln t}{\epsilon_i}
    \end{align*}
    Hence, 
    \begin{align*}
        \probability\left(\eventfive^c\right\Big| \eventone, \eventfour) &\leq \probability\left(\sum_{l = t - v_i(t)}^{t} \left[\service_i(l) - \arrival_i(l)\right] \Big| \eventone, \eventfour\right)\\
        &\leq \exp\left(-\frac{1}{2}\frac{4}{9}\frac{48 \ln t}{\epsilon_i}\right) \\&\leq \frac{1}{t^{10}}
    \end{align*}
    Taking union bound $\forall i$ and using equation \ref{lm_final_busy_period}, completes the proof.
    \begin{equation}
        \probability\left(\eventfive^c\right) \leq \numofserver\left(\frac{1}{t^{10}} + \frac{8}{t^{7}} + \frac{4k_2}{t^3} + \frac{4}{t^4}\right)
    \end{equation}
    \item \textit{Proof of Lemma \ref{lm_tight_bound_p}}\label{prf_lm_tight_bound_p} - \\
    We will first prove this for $\tau = \frac{t}{2}$ and then take union bound for all $\tau \geq \frac{t}{2}$ to complete the proof. We will use a proof technique similar to lemma \ref{lm_p_wt}.
    \begingroup
    \allowdisplaybreaks
    \begin{align*}
        \probability\left(\left|\hat{\mu}_i(\tau) - \mu_i\right|> k_{11}\sqrt{\frac{\ln t}{t}}\Big| \eventone \right) \leq &  \probability\left(\sum_{l=1}^{\tau} \departure_i(l) < n_0\Big| \eventone\right) + \sum_{n=n_0}^{t}\probability\left(\left|\hat{\mu}_i^{(n)} - \mu_i\right|> k_{11}\sqrt{\frac{\ln t}{t}}\Big| \eventone \right)\\
        \leq& \probability\left( \sum_{l=1}^{\tau}\departure_i(l) < n_0 \Big| \sum_{l=1}^{\tau_2}\arrival_i(l) \geq n_0,  \eventone\right) + \probability \left(\sum_{l=1}^{\tau_2} \arrival_i(l) < n_0\Big| \eventone\right) +\\
        &\sum_{n=n_0}^{t}\exp\left( -\frac{k_{11}^2 n c_g \ln t}{t}\right)\\
        \leq& \underbrace{\probability\left( \sum_{l=1}^{\tau}\departure_i(l) < n_0 \Big| \sum_{l=1}^{\tau_2}\arrival_i(l) \geq n_0,  \eventone\right)}_{T_1} + \underbrace{\probability \left(\sum_{l=1}^{\tau/2} \arrival_i(l) < n_0\Big|  \eventone\right)}_{T_2} + \\
        &\underbrace{t\exp\left( -\frac{k_{11}^2 n_0 c_g \ln t}{t} \right)}_{T_3}
    \end{align*}
    \endgroup
    Now choose $\tau_2 = \frac{3t}{8}$ and $n_0 = \frac{p_i^* \lambda t}{32}$. Then,
    \begin{align*}
        \expectation\left(\sum_{l=\frac{t}{4}}^{\frac{3t}{8}}\explore_i(l)\Big| \eventone\right) &\geq \frac{t}{8}\lambda\left( \frac{\ln l}{l} + \left(1 - \frac{\ln l }{l}\right)\hat{p}_i^{(\tau)}\right)\\
        &\geq \frac{t}{8}\lambda\hat{p}_i^{(\tau)}\\
        &\geq \frac{p_i^*\lambda t}{16}\\
    \end{align*}
    Now, bounding $T_2$, we get
    \begin{align*}
        \probability\left(\sum_{l=1}^{\tau_2}\arrival_i(l) < \frac{p_i^*\lambda t}{32}\Big| \eventone\right) &\leq \probability\left(\sum_{l=t/4}^{t/2}\explore_i(l) < \frac{p_i^*\lambda t}{32}t\Big| \eventone\right)\\
        &\leq \exp\left(-\frac{p_i^*\lambda t}{128}\right)
    \end{align*}
    Following a proof similar to that used in lemma \ref{lm_p_wt} and bounding $T_1$, we get,
    \begin{align*}
        \probability\left(\sum_{l=1}^{\tau}\departure_i(l) < \frac{p_i^* \lambda t}{32}\Big| \eventone, \sum_{l=1}^{3t/8}\arrival_i(l) > \frac{p_i^*\lambda t}{32}\right) &\leq \probability \left( \sum_{l=w(t)}^{\frac{t}{2}} \arrival_i(l) < \frac{p_i^*\lambda t}{32}t\Big| \eventone\right)\\
        &\leq \exp\left(-\frac{p_i^*\lambda t}{128}\right)
    \end{align*}
    Using the above expression we get,
    \begin{align*}
        \probability\left(\left|\hat{\mu}_i(\tau) - \mu_i\right| \geq k_1 \sqrt{\frac{\ln t}{t}}\Big| \eventone \right) &\leq \exp\left(-\frac{p_i^*\lambda t}{128}\right) + \frac{1}{t^4}
    \end{align*}
    % \\\\Consider the following events.
    % \begin{equation}
    %     \mathcal{E}_{61} := \sum_{l = w(t)}^{\frac{t}{8}} A_i(l) > \frac{\lambda p_i^* t}{32}.
    % \end{equation}
    % \begin{equation}
    %     \mathcal{E}_{62} := |\hat{\mu}_i^{(n)} - \mu_i| < k_{11}\sqrt{\frac{\ln t}{t}},\> n = \frac{\lambda p_i^* t}{32},
    % \end{equation}
    % where $\hat{\mu}_i^{(n)}$ is the estimate of $\mu_i$ using $n$ independent samples of i.i.d. geometric random variable with parameter $\mu_i$.
    % \begin{equation}
    %     \mathcal{E}_{63} := \mbox{Time to depart $n$ jobs from server $i$} \leq \frac{t}{8}.
    % \end{equation}
    % \begin{equation}
    %     \mathcal{E}_{64} := |\hat{\mu}_i(\tau) - \mu_i| \leq k_{11}\sqrt{\frac{\ln t}{t}},\> k_{11} = \sqrt{\frac{128}{\lambda c_g p_{min}^*}}.
    % \end{equation}
    % Now,
    % \begin{equation}
    %     \mathcal{E}_{64}\Big| \eventone =\mathcal{E}_{61}\cap \mathcal{E}_{62} \cap\mathcal{E}_{63}\Big| \eventone \subseteq \eventsix\Big| \eventone
    % \end{equation}
    % where the last inequality uses lemma \ref{lm_relation_p_mu}. We will now bound each of the term as follows
    % \begin{itemize}
    %     \item  \textit{Bounding probability of event $\mathcal{E}_{61}$} - 
    %     \begin{align*}
    %         \expectation\left(\sum_{l=\frac{t}{4}}^{\frac{3t}{8}}\explore_i(l)\Big| \eventone\right) &\geq \frac{t}{8}\lambda\left( \frac{\ln l}{l} + \left(1 - \frac{\ln l }{l}\right)\hat{p}_i^{(\tau)}\right)\\
    %         &\geq \frac{t}{8}\lambda\hat{p}_i^{(\tau)}\\
    %         &\geq \frac{p_i^*\lambda t}{16}\\
    %     \end{align*}
    %     Now, bounding $T_3$, we get
    %     \begin{align*}
    %         \probability\left(\mathcal{E}_{61}^c\Big| \eventone \right) &\leq \probability \left( \sum_{l=t/4}^{3t/8} \arrival_i(l) < \frac{p_i^*\lambda t}{32}t\Big| \eventone \right) \\
    %         &\leq \probability \left( \sum_{l=t/4}^{3t/8} \explore_i(l) < \frac{p_i^*\lambda t}{32}t\Big| \eventone\right) \\
    %         &\leq \exp\left(-\frac{p_i^*\lambda t}{128}\right)\\
    %         &\leq \frac{1}{t^8}\\
    %     \end{align*}
    %     \item \textit{Bounding probability of event $\mathcal{E}_{62}$} - \\
    %     \begin{align*}
    %         \probability\left( \mathcal{E}_{62}^c\right) &\leq \expectation\left( - c_g \frac{p_i^*\lambda t}{32} k_{11}^2 \frac{\ln(t)}{t} \right)\\
    %         &\leq \expectation\left( - 4\ln t \right)\\
    %         &\leq \frac{1}{t^4}
    %     \end{align*}
    %     \item \textit{Bounding probability of event $\mathcal{E}_{114}$} - \\
    %     Let $X_1, X_2, \cdots, X_n$ be the time taken by the jobs respectively. Now,
    %     \begingroup
    %     \allowdisplaybreaks
    %     \begin{align*}
    %         |\hat{\mu}_i^{(n)} - \mu_i| &\leq k_{11}\sqrt{\frac{\ln t}{t}}\\
    %         \implies \hat{\mu}_i^{(n)} &\geq \mu_i - k_{11}\sqrt{\frac{\ln t}{t}}\\
    %         \implies \sum_i X_i &\leq \frac{\lambda p_i^* t}{32\left(\mu_i - k_{11}\sqrt{\frac{\ln t}{t}}\right)}\\
    %         \implies \sum_i X_i &\overset{(a)}{\leq} \frac{\lambda p_i^* t}{16\mu_i} \leq \frac{t}{8}\\
    %         \implies \mbox{Time taken to depart $n$ jobs} &\leq \frac{t}{8}\\
    %         \implies \mathcal{E}_{62} &\subseteq \mathcal{E}_{63}
    %     \end{align*}
    %     \endgroup
    %     where $(a)$ follows from the definition of $\Delta_0, t_0$
    % \end{itemize}
    % This gives, 
    % \begin{equation}
    %     \probability\left(\eventsix^c \Big | \eventone\right) \leq  \probability\left(\mathcal{E}_{64}^c\Big | \eventone\right) \leq \probability\left(\mathcal{E}_{61}\Big | \eventone^c\right) + \probability\left(\mathcal{E}_{62}^c\right) +  \probability\left(\mathcal{E}_{63}^c\right) \leq \frac{2}{t^4} + \frac{1}{t^8}
    % \end{equation}
    % Now,
    % \begin{align*}
    %     \probability\left(\eventsix^c\right\Big| \eventone) \leq& \underbrace{\probability\left(\eventsix^c\Big| \eventone, \numberofevents_{\departure_i}\left(\frac{t}{2}\right) > \frac{p_i^*\lambda t}{32} \right)}_{t_1} + \underbrace{\probability\left(\numberofevents_{\departure_i}\left(\frac{t}{2}\right) < c_1t\Big| \eventone, \numberofevents_{\arrival_i}\left(\frac{3t}{8}\right) > \frac{p_i^*\lambda t}{32} \right)}_{T_1} +\\
    %     &\underbrace{\probability\left(\numberofevents_{\arrival_i}\left(\frac{3t}{8}\right) < \frac{p_i^*\lambda t}{32}\Big| \eventone\right)}_{T_3}
    % \end{align*}
    % Now, 
    % \begin{align*}
    %     \expectation\left(\sum_{l=\frac{t}{4}}^{\frac{3t}{8}}\indicatorofevents_{\explore_i}(l)\Big| \eventone\right) &\geq \frac{t}{8}\lambda\left( \frac{\ln l}{l} + \left(1 - \frac{\ln l }{l}\right)\hat{p}_i^{(\tau)}\right)\\
    %     &\geq \frac{t}{8}\lambda\hat{p}_i^{(\tau)}\\
    %     &\geq \frac{p_i^*\lambda t}{16}\\
    % \end{align*}
    % Now, bounding $T_3$, we get
    % \begin{align*}
    %     \probability\left(\numberofevents_{\arrival_i}\left(\frac{3t}{8}\right) < \frac{p_i^*\lambda t}{32}t\Big| \eventone\right) &\leq \probability\left(\sum_{l=w(t)}^{\frac{t}{2}}\indicatorofevents_{\arrival_i}(l) < \frac{p_i^*\lambda t}{32}t\Big| \eventone\right)\\
    %     &\leq\probability\left(\sum_{l=\frac{t}{4}}^{\frac{t}{2}}\indicatorofevents_{\explore_i}(l) < \frac{p_i^*\lambda t}{32}t\Big| \eventone\right)\\
    %     &\leq \exp\left(-\frac{p_i^*\lambda t}{128}\right)
    % \end{align*}
    % Similarly, bounding $T_2$, we get,
    % \begin{align*}
    %     \probability\left(\numberofevents_{\departure_i}\left(\frac{t}{2}\right) < c_1t\Big| \eventone, \numberofevents_{\arrival_i}\left(\frac{3t}{8}\right) > \frac{p_i^*\lambda t}{32}\right) &\leq \probability \left( \sum_{l=w(t)}^{\frac{t}{2}} \indicatorofevents_{\arrival_i}(l) < \frac{p_i^*\lambda t}{32}t\Big| \eventone\right)\\
    %     &\leq\probability\left(\sum_{l=\frac{t}{4}}^{\frac{t}{2}}\indicatorofevents_{\explore_i}(l) < \frac{p_i^*\lambda t}{32}t\Big| \eventone\right)\\
    %     &\leq \exp\left(-\frac{p_i^*\lambda t}{128}\right)
    % \end{align*}
    % \Tuhin{Have to Use proper notation of service}
    % Finally, bounding $T_1$, we get
    % \begin{align*}
    %     \probability\left(\left|\hat{p}_i^{(\tau)} - p_^*\right| \geq k_1 \sqrt{\frac{\ln t}{t}}\Big| \eventone, \numberofevents_{\departure_i}\left(\frac{t}{2}\right) > \frac{p_i^*\lambda t}{32} \right) &\leq \expectation\left( - c_g \frac{p_i^*\lambda t}{32} k_1^2 \frac{\ln(t)}{t} \right)\\
    %     &\leq \expectation\left( - 4\ln t \right)\\
    %     &\leq \frac{1}{t^4}
    % \end{align*}
    Taking an union bound $\forall \tau \in \left(\frac{t}{2}, t\right)$ and using lemma \ref{lm_p_wt}, we get
    \begin{equation}
        \probability\left(\eventsix^c\right) \leq \probability\left(\eventsix^c\Big|\eventone\right) + \probability\left(\eventone^c\right) \leq \numofserver\left(\frac{1}{t^7} + \frac{k_2}{t^3} + \frac{1}{t^3} + t \exp\left(-\frac{p_i^*\lambda t}{128}\right)\right)
    \end{equation}
    \item \textit{Proof of equation \ref{rel_diff_p}}\label{prf_rel_diff_p} - \\
    We will define the following terms.
    \begin{equation}
        common_i(t) = common_i^*(t) = \min\left\{\hat{p}_i(t), p_i^*\right\}, \forall i.
    \end{equation}
    \begin{equation}
        residual_i(t) = \max\left\{\hat{p}_i(t) - p_i^*, 0\right\}, \forall i.
    \end{equation}
    \begin{equation}
        residual_i^*(t) = \max\left\{p_i^* - \hat{p}_i(t), 0\right\}, \forall i.
    \end{equation}
    Assume, $common_i(t) = residual_i(t) = \sum_i common_i^*(t) = residual_i^*(t) = 0, \forall i \notin [1, K]$. It is easy to show that 
    \begin{equation}
        \sum_i common_i(t) + residual_i(t) = \sum_i common_i^*(t) + residual_i^*(t) = 1
    \end{equation}
    Also, observe that for all $i$,
    \begin{equation}
        \min\left\{residual_i(t), residual_i^*(t)\right\} = 0.
    \end{equation}
    For system following the optimal policy $\policy^*$, divide the region $0-1$ into $2\numofserver$ sub-regions, where the sub-regions namely $sub_1^*(t), sub_2^*(t), \cdots, sub_{2\numofserver}^*(t)$ such that 
    \begin{equation}
        sub_i^*(t) := \left[\sum_{j = 0}^{i-1} common_i^*(t), \sum_{j = 0}^{i} common_i^*(t)\right), \forall i \leq \numofserver,
    \end{equation}
    \begin{equation}
        sub_{\numofserver + i}^*(t) := \left[\sum_{j = 0}^{\numofserver} common_i^*(t) + \sum_{j = 0}^{i-1} residual_i^*(t), \sum_{j = 0}^{\numofserver} common_i^*(t) + \sum_{j = 0}^{i} residual_i^*(t)\right), \forall i \leq \numofserver.
    \end{equation}
    Similarly, for the system following policy $\policy$, divide the region $0-1$ into $2\numofserver$ sub-regions, where the sub-regions namely $sub_1(t), sub_2^*(t), \cdots, sub_{2\numofserver}^*(t)$ such that 
    \begin{equation}
        sub_i(t) := \left[\sum_{j = 0}^{i-1} common_i(t), \sum_{j = 0}^{i} common_i(t)\right), \forall i \leq \numofserver,
    \end{equation}
    \begin{equation}
        sub_{\numofserver + i}(t) := \left[\sum_{j = 0}^{\numofserver} common_i^*(t) + \sum_{j = 0}^{i-1} residual_i(t), \sum_{j = 0}^{\numofserver} common_i(t) + \sum_{j = 0}^{i} residual_i(t)\right), \forall i \leq \numofserver.
    \end{equation}
    Now, the coupling works as follows, 
    \begin{enumerate}
        \item Every incoming job generates a common random variable $U\sim Unif[0, 1]$.
        \item For the system following $\policy^*$, the job is sent to server $i$ through exploitation, if $U\in sub_i^*(t)$ or $U\in sub_{\numofserver + i}^*(t)$.
        \item For the system following $\policy$, the job is sent to server $i$ through exploitation, if $U\in sub_i(t)$ or $U\in sub_{\numofserver + i}(t)$, given $\explore_i(t) = 1$.
    \end{enumerate}
    Now, 
    \begin{align}
        \expectation\left[\indicatorofevents_{ \{\exploit_i(l) \neq \exploit_i^*(l)\}} \right] &\leq \expectation\left[U \in sub_i^*(t)\cup U \in sub_i(t) \right]\\
        &\leq \expectation\left[U \in sub_i^*(t)\right] +  \expectation\left[U \in sub_i(t) \right]\\
        &\leq residual_i^*(t)+ residual_i(t)\\
        &\leq |\hat{p}_i(t) - p_i^*|
    \end{align}
\end{enumerate}
